# Supplementary material for: Chiral states in coupled-lasers lattice by on-site complex potential
Source: arXiv:2109.08085 source file (2021-09-21)
Supplement: Supplementary file 1 [file Chirality_by_complex_potential-_Supplementary_material.pdf]

# Chiral states in coupled-lasers lattice by on-site complex potential - Supplementary material

Sagie Gadasi[†], Geva Arwas[†], Igor Gershenzon, Asher Friesem and Nir Davidson
*Department of Physics of Complex Systems, Weizmann Institute of Science, Rehovot 7610001, Israel*

## DETAILED EXPERIMENTAL SETUP DESCRIPTION

The detailed experimental arrangement of the digital degenerate ring cavity laser (DDRCL) [1] is schematically presented in figure S1(a). The DDRCL includes a gain medium, two 4f telescopes with one common lens, a reflective phase only spatial light modulator (SLM), two retroreflectors and pentaprism-like 90 degree reflector (all from high reflectivity mirrors), two polarizing beam splitters (PBS), two half-wave plates ($\lambda/2$) and a Faraday rotator.

The laser gain medium was a 1.1% doped Nd-YAG rod of 10-mm diameter and 11-cm length. For quasi-CW operation, the gain medium was pumped above threshold by a 200$\mu s$ pulsed xenon flash lamp operating at 1800-1950V and a repetition rate of 1 Hz to avoid thermal lensing. Each 4f telescope consists of two plano-convex lenses, with diameters of 50.8$mm$ and focal lengths of $f_1 = 750mm$ and $f_1 = 500mm$ at the lasing wavelength of 1064$nm$. The SLM was Meadowlark (liquid crystal on silicon (LCOS)) with a zero order diffraction efficiency of 88%, an area of 17.6$mm$ by 10.7$mm$, 1920 by 1152 resolution, 9.2$\mu m$ pixel size, and a high damage threshold ($200\frac{W}{cm^2}$).

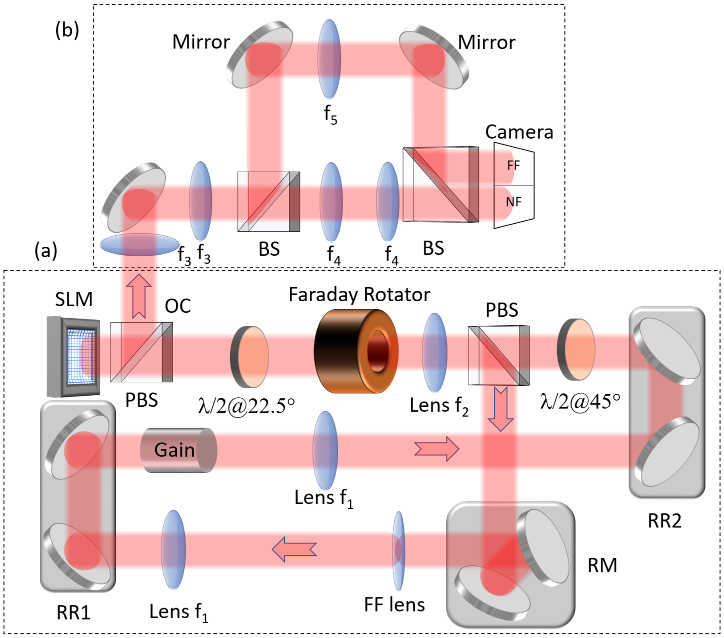


FIG. S1: Schematic drawing of the experimental setup. (a) Folded digital degenerate ring cavity laser, supporting the two laser. (b) Interferometer for intensity and phase measurements.

In the DDRCL, each of the two 4f telescopes has one lens f1 and a common lens f2. The first telescope images the field distribution at the center of the gain medium onto the SLM where the reflectivity of each effective pixel is controlled [2]. The second telescope, images the field distribution at the SLM back onto the gain medium. The coupling is done inserting a lens with focal length of 5m to the Fourier plane of the second telescope (FF lens in the drawing). Since the SLM operates on axis and by reflection on horizontal polarized light, half of the ring degenerate cavity was designed as a twisted-mode [3] linear degenerate cavity [4] and the other half as regular ring cavity laser. The two halves are connected by PBS1, which separates the two counter-propagating beams into two

different cross-polarized paths. A large aperture Faraday another PBS2 (which also serves as $\sim 5\%$ output coupler) enforce unidirectional operation of the DDRCL. A 90° reflector flips left and right areas of the beam. A second HWP at 45° rotates the polarization from vertical to horizontal to pass through PBS1.

The detection arrangement is shown in S1(b), and includes a CMOS camera, lenses, and beam splitters. The laser's output is split into two channels: one for imaging the near-field and the other for imaging the far-field.

The local reflectivity magnitude of the SLM is determined by local phase differences between adjacent pixels and affects the amount of light diffracted out of the cavity. The local reflectivity phase is determined by the local average phase of the adjacent pixels [2]. For example, adjacent pixels with phases of $[0, 0]$ will result in high reflectivity and 0 phase, whereas adjacent pixels with phases of $[0, \pi]$ will result in no reflectivity and $\frac{\pi}{2}$ phase. The SLM enables the generation of lasers arrays with arbitrary geometries, and to control to loss and frequency detuning of each of the lasers individually arbitrary loss and phase distribution, and it is used to create the lasers, and to add relative loss and detuning between them [5].

### Experiment parameters

The cavity round-trip time is $\tau_c \approx 17$ns and corresponds to free spectral range of $FSR \approx 60$MHz. The estimated values of the round-trip unsaturated gain at the lasing threshold are $g_{th,lattice} \approx 2.55$ and $g_{th,triangle} \approx 5.05$ for lasers in a triangular lattice and in a single triangle (ring of three lasers) correspondingly. From these values, we can caclulate the magnitude of the coupling coefficient $\kappa$ and the round-trip loss of an individual laser $\alpha_0$, according to the following coupled equations:

$$g_{th,lattice} = \alpha_0 - [6 \cdot (-\kappa) \cdot \cos(\frac{2\pi}{3})] \tag{S1}$$

$$g_{th,triangle} = \alpha_0 - [2 \cdot (-\kappa) \cdot \cos(\frac{2\pi}{3})] \tag{S2}$$

where the prefactor of the coupling 6 and 2 are the number of nearest neighbors. Using the estimated values for $g_{th,lattice}$ and $g_{th,triangle}$, we find that $\kappa = 1.25$ and $\alpha_0 = 6.3$. In units of frequencies, the coupling coefficient is $\kappa = 75MHz$.

## LASER RATE EQUATIONS AND COLD-CAVITY MODES

The starting point of the analysis are the laser rate equations (LRE), which describe the dynamics of N single-mode class-B coupled lasers [6]:

$$\frac{dG_m}{dt} = \frac{1}{\tau_f}\left[g_{0,m} - G_m\left(1 + \frac{|E_m|^2}{I_{sat}}\right)\right] \tag{S3}$$

$$\frac{dE_m}{dt} = \frac{1}{\tau_c}\left[\left(G_m - \alpha_m\right)E_m + \sum_{n\neq m}\kappa_{mn}E_n\right] + i\Omega_m E_m\,, \tag{S4}$$

where $E_m$ and $E_n$ are the complex electric fields of the laser $m$ and laser $n$, $G_m$ and $g_{0,m}$ are the gain and unsaturated gain of the $m$'th laser, $I_{sat}$ the saturation intensity, $\alpha_m$ the $m$'th laser loss, $\Omega_m$ the $m$'th laser resonator-frequency and $\kappa_{nm}$ the coupling between laser $n$ and laser $m$. The fluorescence time of the gain medium and the cavity round-trip time are given by $\tau_f$ and $\tau_c$.

### Cold cavity modes

The cold cavity modes (CCM) dynamics can be found by setting the gain to zero $g_0 = 0$. Then, the equations of motion are reduced to

$$\frac{dE_m}{dt} = -\frac{1}{\tau_c}\alpha_m E_m + \frac{1}{\tau_c}\sum_{n\neq m}\kappa_{mn}E_n + i\Omega_m E_m\,.$$

This equations can be rewritten in as:

$$i\frac{d}{dt}\boldsymbol{E} = \left(\Omega_0 + \alpha_0\right)\mathbb{I}\boldsymbol{E} + \mathcal{H}\boldsymbol{E}$$

where $\boldsymbol{E}$ is a column vector of the electric field in the cavities and, $\Omega_0$ and $\alpha_0$ are the average frequency and average loss of the cavities, and $\mathcal{H}$ is the effective Hamiltonian. The diagonal entries of $\mathcal{H}$ are the loss differences $\{\Delta\alpha_m\}$ and frequency differences $\{\Delta\Omega_m\}$ of the different cavities from the average values. The off-diagonal entries of $\mathcal{H}$ are the coupling coefficients between the cavities. In our system the coupling coefficients are identical and symmetric, hence $\kappa_{mn} = \kappa$.

For example, a system of three negatively coupled lasers with the loss and frequency detuning displayed in figure S2 will be described by the following Hamiltonian:

$$\mathcal{H} = \begin{pmatrix} -\frac{1}{2}\Delta\Omega & -i\kappa & -i\kappa \\ -i\kappa & -i\Delta\alpha & -i\kappa \\ -i\kappa & -i\kappa & +\frac{1}{2}\Delta\Omega \end{pmatrix}. \tag{S5}$$

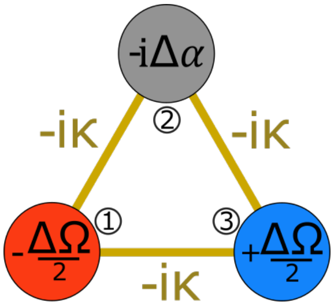


FIG. S2: Three negatively coupled laser with a complex potential. A loss of $\Delta\alpha$ is applied to the apex laser (laser 2) and a frequency detuning of $\pm\frac{1}{2}\Delta\Omega$ is applied to the base lasers (laser 1 and 3).

## ANTI-PT SYMMETRIC HAMILTONIAN

The Hamiltonian in equation (S5) is anti-PT-symmteric [7], i.e. it anti-cummutes with the PT operator. The real and imaginary parts of its eigenvalues for a fixed $\Delta\alpha$ and varying $\Delta\Omega$ are plotted in figure 3 panels (a) and (b) of the main text. The eigenmodes (CCM) at selected points are presented in figure (S3). The first and second rows display the minimal loss and second-minimal-loss CCM.

An EP occurs at $\Delta\Omega_{EP} = 1.1\Delta\alpha$, where the two CCM coalesce into a mode which is a nearly pure vortex or antivortex mode (with a small component of uniform phase mode). For detuning values $\Delta\Omega \leq \Delta\Omega_{EP}$, the system is in the anti-PT-exact phase, at which the amplitudes of the CCM exhibit the same symmetry as the imaginary part of the complex potential (the base lasers have the same amplitude). For detuning values $\Delta\Omega > \Delta\Omega_{EP}$ the system is in the anti-PT broken phase, where the symmetry is broken and the base lasers don't have the same amplitude.

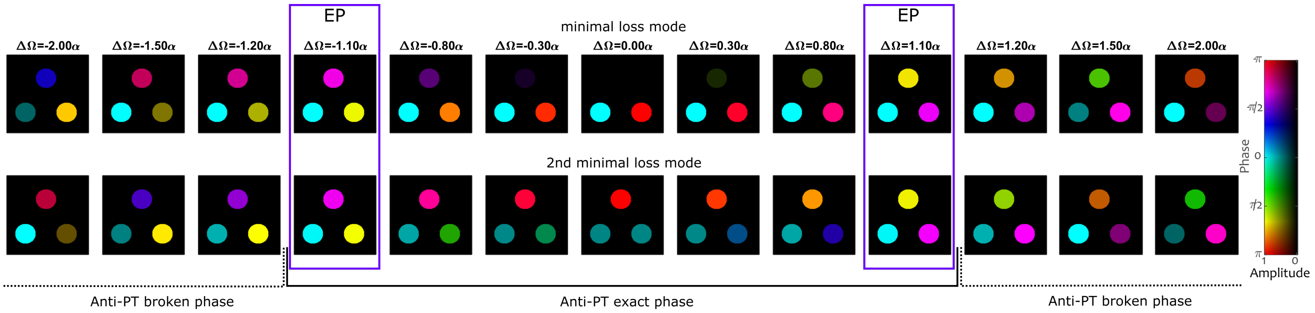


FIG. S3: Illustration of the cold cavity modes for $\Delta\alpha/\kappa = 0.12$ and varying $\Delta\Omega$. The first and second rows display the minimal loss and second minimal loss cold cavity modes. The color hue represents the relative phase $\phi$ and the brightness represents the lasers' amplitude. For $|\Delta\Omega| < \Delta\Omega_{EP}$ , the system is in the anti-PT exact phase, where the two base lasers have equal intensities. At the EP, the two eigenmodes colapse into either vortex or antivortex modes. For $|\Delta\Omega| > \Delta\Omega_{EP}$ , the system is in the anti-PT broken phase, where the two base lasers have different intensities.

## EP DEPENDENCE ON APEX LOSS

The exact frequency detuning value of the exceptional point $\Delta\Omega_{EP}$ depends on the ratio between the coupling coefficient and the relative loss between the lasers $\frac{\Delta\alpha}{\kappa}$. The following figure displays the dependence of $\Delta\Omega_{EP}$ on $\frac{\Delta\alpha}{\kappa}$, obtained by numerical calculation.

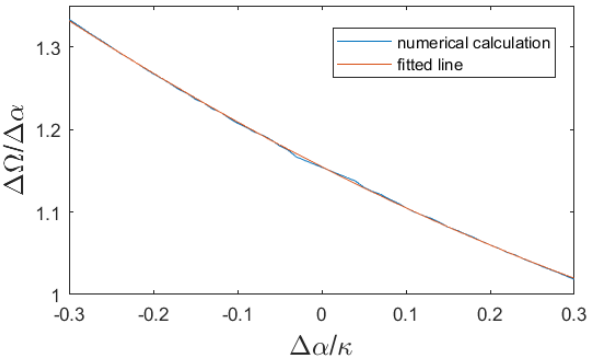


FIG. S4: Numerical calculation of the dependence of the EP location on the ratio $\frac{\Delta\alpha}{\kappa}$.

## NUMERICAL SIMULATION OF THE FULL LRE

To simulate the coupled-laser system, we numerically solved the LRE for three negatively coupled laser. The parameters that we used are similar to the experimental parameters: $\alpha_0 = 6.3$, $\kappa = -1.25$. We used pump value $g_0 = 1.2 \cdot g_{0,th}$, where $g_{0,th}$ is the unsaturated gain at the lasing threshold calculated from the cold cavity Hamiltonian. Since the ratio of $\tau_f$ and $\tau_c$ does not effect the steady state of the laser network, we used $\tau_f = 2\tau_c$ to reduce the calculation time. The values of $\Delta\alpha$ and $\Delta\Omega$ where scanned in the ranges $[-0.2, 0.2]$ and $[-0.3, 0.3]$ correspondingly in steps of 0.01. Each $(\Delta\alpha, \Delta\Omega)$ point was averaged over 5000 realizations. Each realization began with random initial conditions.

The average chirality is presented in figure S5(a). In figure S5(b) we present a scatter plot of the chirality values of all the different realizations. We learn from these plot the the in each $(\Delta\alpha, \Delta\Omega)$ there are two stable fixed point: the vortex and antivortex mode. When the values of $(\Delta\alpha, \Delta\Omega)$ are scanned, the probability to get one mode over the other is changed. For example, zero average chirality means that the system has equal probability to get to a fix point of vortex or antivortex.

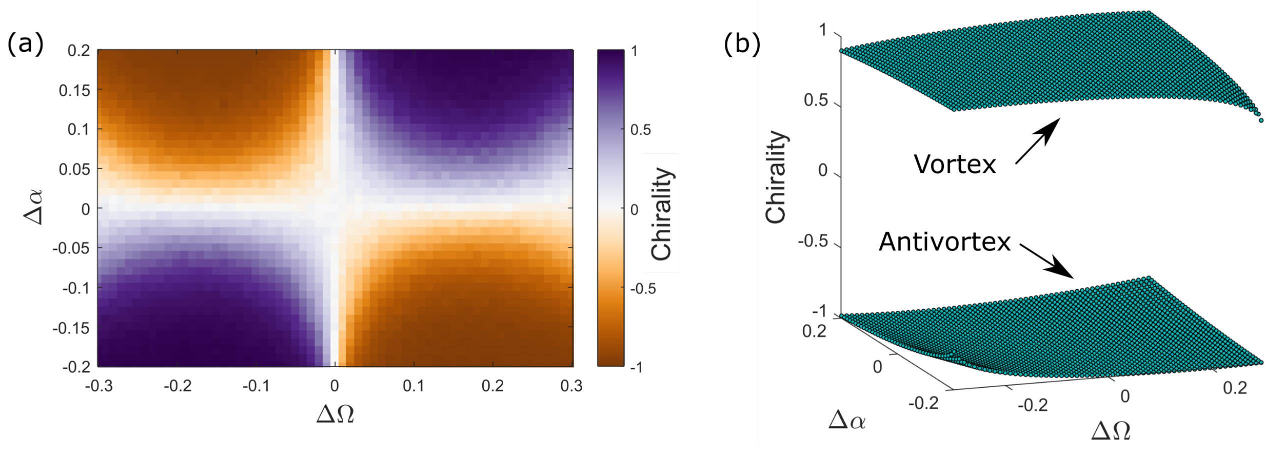


FIG. S5: The chirality of a triangle system, obtained by numerical simulations. For each $(\Delta\alpha, \Delta\Omega)$ point, 5000 repetitions were carried out. (a) Average chirality. (b) Scatter plot of the chirality of all the realizations. While the average chirality at each point of $(\Delta\alpha, \Delta\Omega)$ can take any value between -1 and 1, the chirality of each realization can take one of two values, which are approximately $\pm 1$. For extreme values of $\Delta\alpha$ and $\Delta\Omega$ (which we did not get to in the experiment), the lasing mode deviates significantly from vortex or antivortex and hence the chirality takes absolute values that are significantly smaller than one.

In figure S6 we display the normalizerd difference in the amplitude between laser 2 and 3 to laser 1: $\Delta A_{12} = \frac{|A_1|-|A_2|}{|A_1|+|A_2|}$ and $\Delta A_{13} = \frac{|A_1|-|A_3|}{|A_1|+|A_3|}$. Each point in the plot corresponds to a single realization. We see that the amplitudes of the base lasers always equal $\Delta A_{13} = 0$. This indicates that the system never gets to the anti-PT broken phase. The amplitude difference between the apex and base lasers depend on the values of $\Delta\alpha$ and $\Delta\Omega$, and it is less than 10% within the experimental parameters.

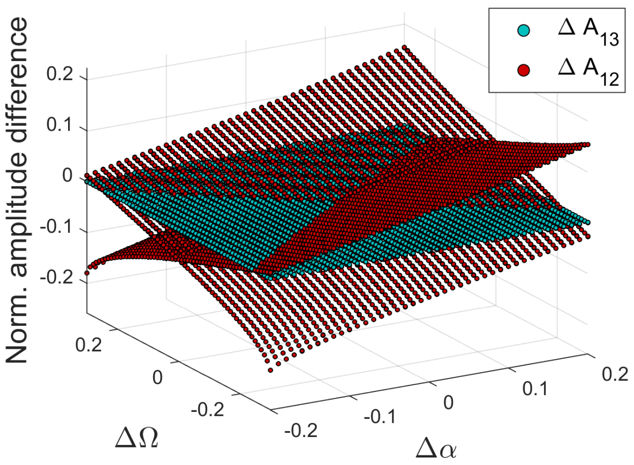


FIG. S6: Simulation results for the normalized amplitude difference between the lasers in steady state. The result of all the realizations are displayed in a scatter plot. $\Delta A_{12}$ is the normalized amplitude difference between the base laser and and the apex laser and $\Delta A_{13}$ is the normalized amplitude difference between the two base lasers. The base lasers have equal amplitudes throughout the scan. The amplitude difference between the apex and base laser does not exceed 10% within the experimental parameters.

## EFFECTIVE LOSS

To understand the effect of saturation on the system in terms of the linear analysis and the EPs, we consider the effective Hamiltonian of the system in steady-state, after the amplitudes of the lasers are known. By definition, the state of the system (the amplitudes of the lasers) must be an eigenmode of the following Hamiltonian:

$$\mathcal{H} = \begin{pmatrix} -\frac{1}{2}\Delta\Omega + i\frac{g_0}{1+|E_1|^2} & -i\kappa & -i\kappa \\ -i\kappa & -i\Delta\alpha + i\frac{g_0}{1+|E_2|^2} & -i\kappa \\ -i\kappa & -i\kappa & +\frac{1}{2}\Delta\Omega + i\frac{g_0}{1+|E_3|^2} \end{pmatrix}$$

We use the observation that the amplitudes of laser 1 and 3 are equal (from the simulation results in previous section) to obtain the following traceless Hamiltonian

$$\mathcal{H} = \begin{pmatrix} -\frac{1}{2}\Delta\Omega & -i\kappa & -i\kappa \\ -i\kappa & -i\Delta\alpha_T & -i\kappa \\ -i\kappa & -i\kappa & +\frac{1}{2}\Delta\Omega \end{pmatrix}$$

with

$$\Delta\alpha_T = \Delta\alpha - \Delta G \tag{S6}$$

and

$$\Delta G = \frac{g_0}{1+|E_2|^2} - \frac{g_0}{1+|E_1|^2}\,,$$

where $\Delta G$ is the nonlinear gain difference between the apex laser (laser 2) and the base lasers (lasers 1 and 3). $\Delta\alpha_T$ is the effective loss between laser 2 and the other lasers in steady state.

The simulation results presented in figure S7 (next page) reveal that the effective loss $\Delta\alpha_{\text{eff}}$ is exactly the loss that is required to bring the system to an EP for the applied detuning ($\Delta\alpha_{\text{EP}}$). The value of $\Delta\alpha_{\text{eff}}$ is displayed as a function of the applied $\Delta\alpha$ for various $\Delta\Omega$ and $g_0$. The red circles display $\Delta\alpha_{\text{eff}}$, and their diameter represent their prevalence among the 5000 realizations. The prevalence is also shown by the ensemble average $\langle\Delta\alpha_{\text{eff}}\rangle$ (dashed line). As explained in the text, the steady-state value of $\Delta\alpha_{\text{eff}}$ approaches the value of $\Delta\alpha_{\text{EP}}$ (dotted line).

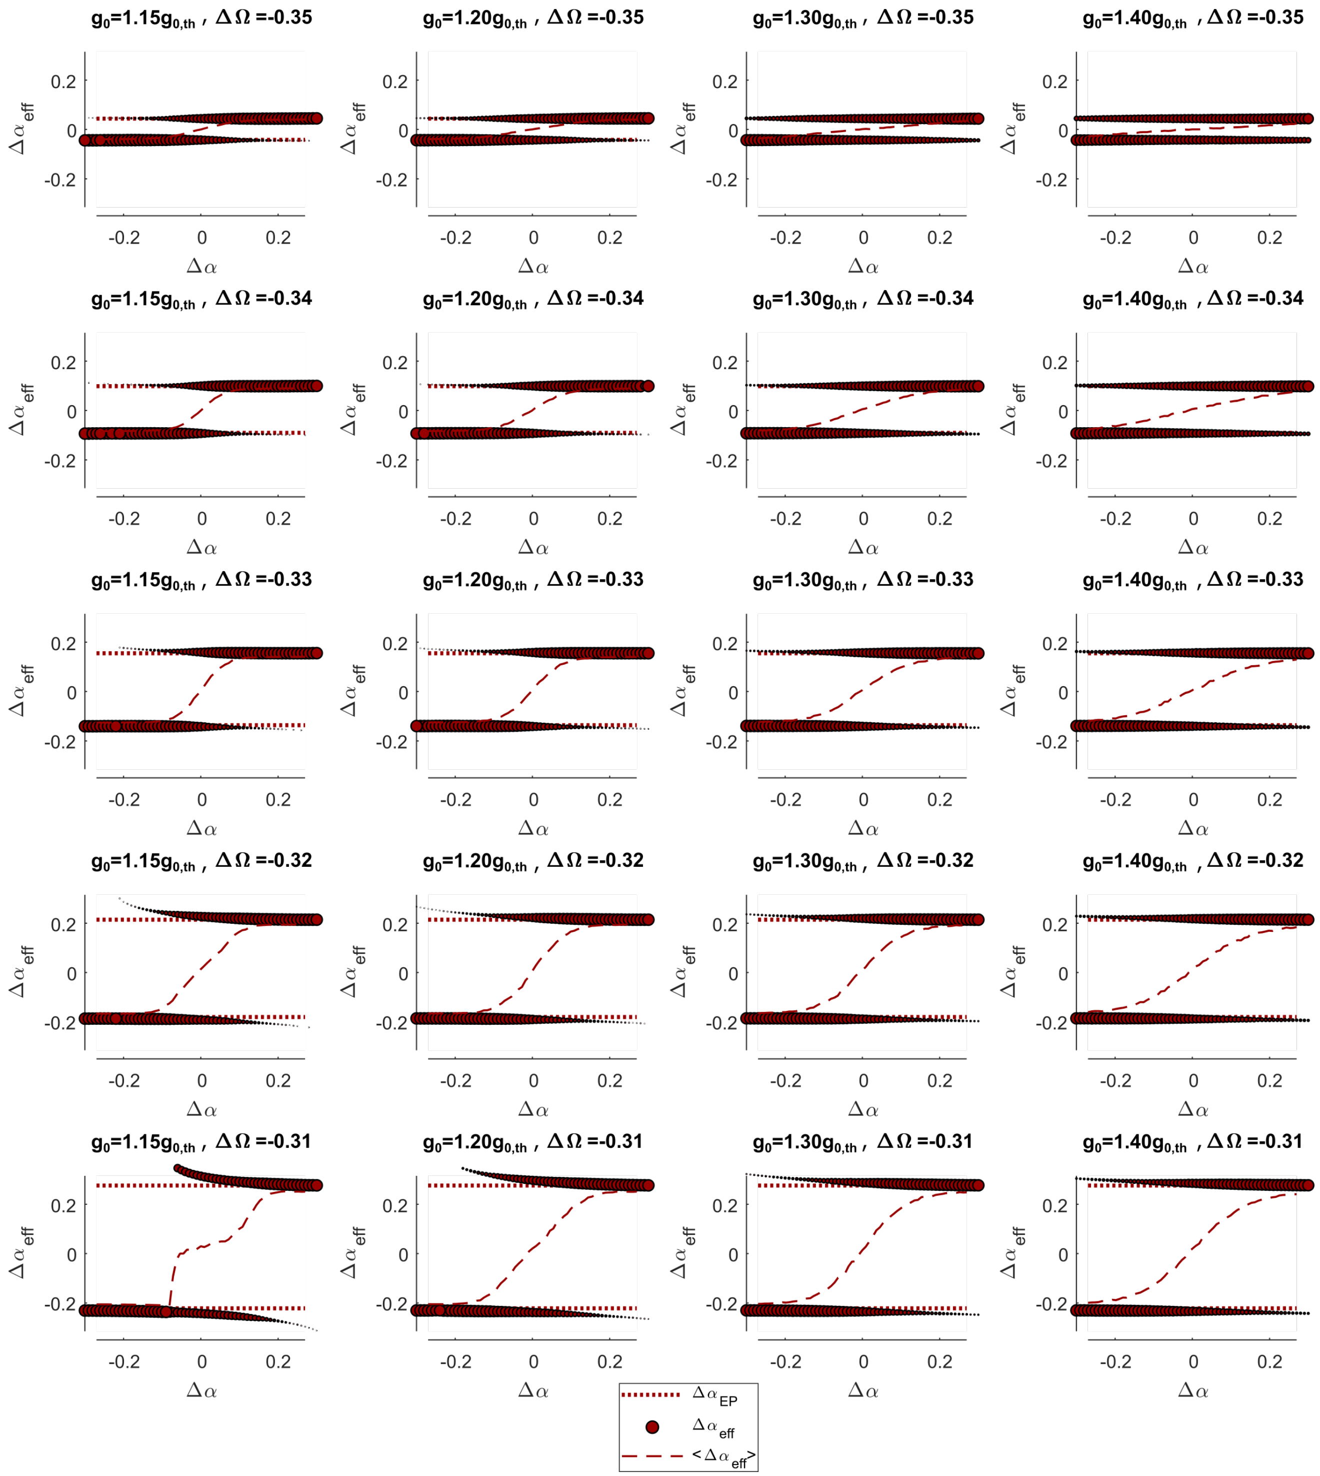


FIG. S7: Simulation results for the effective loss $\Delta\alpha_{\rm eff}$ (red circles) as a function of the applied loss $\Delta\alpha$ for different values of $\Delta\Omega$ and unsaturated gain $g_0$ in units of the gain at the lasing threshold $g_{0,th}$. The circles' diameter represents the prevalence of $\Delta\alpha_{\rm eff}$ among the 5000 realizations. The dashed line shows an ensemble average $\langle\Delta\alpha_{\rm eff}\rangle$. It is clearly seen that the steady-state $\Delta\alpha_{\rm eff}$ approaches the values of $\Delta\alpha_{\rm EP}$ (dotted lines). This demonstrates the effect that the nolinearity of the lasers pulls the system to the EPs. As the pumping rate is increased, larger values of $\Delta\alpha$ are required for the system to well distinguish between the two modes.

## TWO LASERS: PHASE-DIRECTIONALITY BY FREQUENCY DETUNING

In this section we show that if that two detuned lasers have aphase difference that depends on their detuning. are added can be found in what follows. By defining $E_m = A_m e^{i\phi_m}$, we can rewrite the LRE in the following way:

$$\frac{dA_m}{dt} = \frac{1}{\tau_c}\left(G_m - \alpha_m\right) A_m\left(t\right) + \sum_{n\neq m} \frac{\kappa_{nm}}{\tau_c} A_n\left(t\right)\cos\left(\phi_n\left(t\right) - \phi_m\left(t\right)\right)\ , \tag{S7}$$

$$\frac{d\phi_m}{dt} = \Omega_m + \sum_{n\neq m} \frac{\kappa_{nm}}{\tau_c}\frac{A_n\left(t\right)}{A_m\left(t\right)}\sin\left(\phi_n\left(t\right) - \phi_m\left(t\right)\right)\ . \tag{S8}$$

where $A_m$ is the amplitude of the electric field and $\phi_m$ is the phase of the $m$'th laser.

At steady state, after the amplitudes have settled, for uniform negative coupling, the phases of the lasers are described by the following equation:

$$0 = \Omega_m - \kappa \sum_{n\neq m} \frac{A_n}{A_m}\sin\left(\phi_n - \phi_m\right)\ .$$

If we assume that the two lasers have the same amplitude, and that they are detuned by $\Delta\Omega$, their phase difference is given by

$$\sin\left(\phi_2 - \phi_1\right) = \frac{\Omega_1 - \Omega_2}{2\kappa}\ .$$

The laser with the lower frequency leads in phase.

## THREE LASERS: CHIRALITY BY FREQUENCY DETUNING

In this section we demonstrate the importance of a combination of loss and frequency detuning, a complex potential, in inducing chirality in a three negatively-coupled oscillators system. To do that, we ask: can we induce chirality to the system by some combination of frequency detuning between the three oscillators? We consider a system of three frequency-detuned, negatively coupled oscillators such that the second and third oscillators are detuned by $\Delta\Omega_1$ and $\Delta\Omega_2$ from the first oscillator ans we examine three kinds of oscillators: linear oscillators (coupled cavities: lasers without pumping), phase oscillators (Kuramoto model) and lasers with various pumping rates. In all cases, the chirality was calculated according to equation (1) in the main paper.

The Linear system, is descirbed by the following effective Hamiltonian:

$$\mathcal{H} = \begin{pmatrix} 0 & -i\kappa & -i\kappa \\ -i\kappa & \Delta\Omega_1 & -i\kappa \\ -i\kappa & -i\kappa & \Delta\Omega_2 \end{pmatrix}.$$

Figure S8(a) displays the chirality of the minimal loss eigenmode of $\mathcal{H}$, calculated from its projection on the vortex and antivortex modes. We observe that if only one laser is frequency-detuned, no chirality is induced. If a combination of $\Delta\Omega_1$ and $\Delta\Omega_2$ is applied, we see that an extremely small chirality is induced ($c < 0.02$, note the different colorbar range).

For phase oscillators, the system dynamics is given by equation S8, with the constraints of equal amplitude (and therefore the equation reduces to the simple Kuramoto model). Figure S8(b) displays the average chirality of the steady state solution of three negatively-coupled phase oscillators, where each point is averaged over 100 realizations. From these results we learn that frequency detuning alone cannot induce chirality.

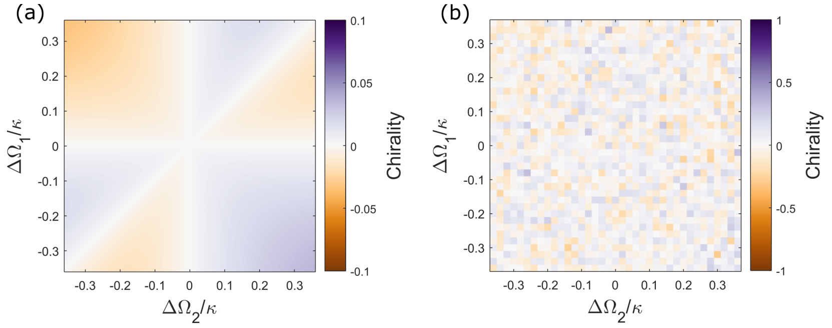


FIG. S8: (a) Chirality of a system of linear coupled oscillators, calculated from the minimal loss eigenmode of $\mathcal{H}$. (b) Average chiraity of a system of coupled phase oscillators, calculated from numerical simulations of equation S8. For both linear oscillators and phase oscillators, detuning alone is not sufficient to induce significant chiarality to the system.

For a system of coupled lasers, we solved the LRE numerically for 3 different unsaturated gain values, and the results for the average chirality are presented in figures S9(a)-(c). All the other system parameters are identical to those used in previous sections. We see that when only one of the lasers is frequency detuned ($\Delta\Omega_1 = 0$ or $\Delta\Omega_2 = 0$), no chirality is induced. Nevertheless, when the sum of $\Delta\Omega_1$ and $\Delta\Omega_2$ exceeds a certain value (that depends on the pumping rate), strong chirality is induced. We see that when the pumping rate is larger, larger detuning values are required for inducing chirality. Figures S9(d)-(f) display the inhomogeneity of the lasers amplitude $\frac{|A|_{max}-|A|_{min}}{|A|_{max}}$, as a function of the $\Delta\Omega_1$ and $\Delta\Omega_2$. $|A|_{max}$ and $|A|_{min}$ are the absolute value of the amplitude of the strongest laser and weakest lasers. For comparison, figures S10 display the simulation results for laser system with the exact same parameters but with complex potential. By comparing figure S9 and figure S10 we learn that complex potential enable to induce chirality with frequency detuning that is much smaller than in the case of detuning-only. Also, by comparing the figures that present the amplitude difference, we see that the inhomogeneity of the laser amplitude

is much larger when the detuning-only approach is used. Furthermore. when the complex potential is tuned to the EP, the lasers amplitude are nearly identical, producing more pure vortex modes.

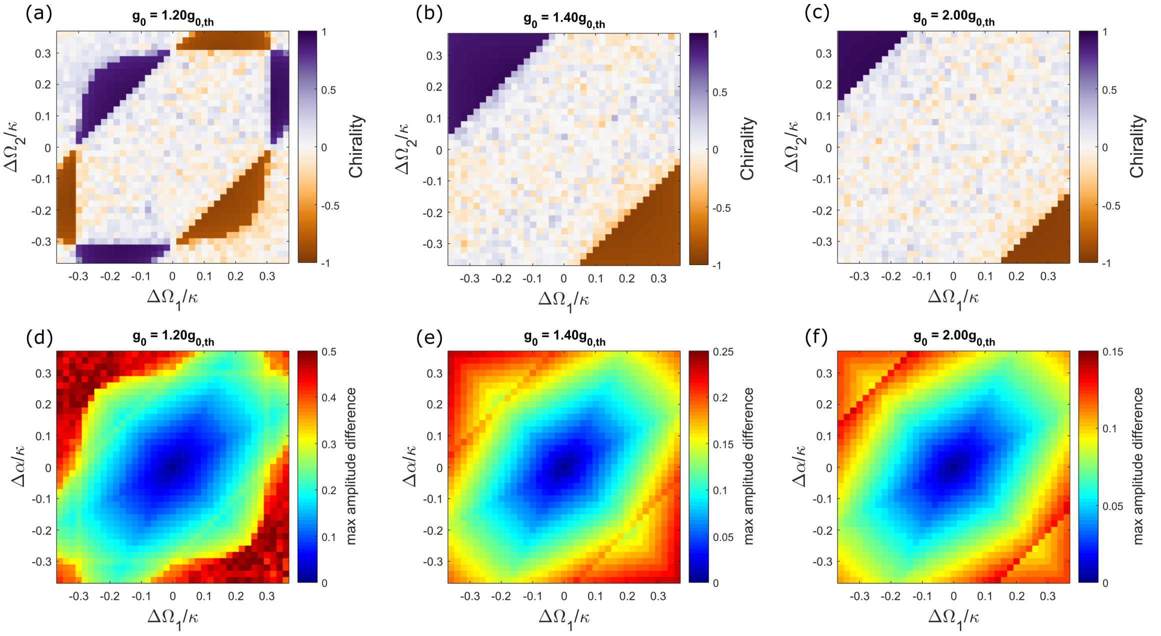


FIG. S9: (a) Chirality and (b) amplitude inhomogeneity of a system of coupled lasers as a function of $\Delta\Omega_1$ and $\Delta\Omega_2$, calculated by numerically solving the LRE for variuos values of $g_0$. Note the different colorbar range in panels (d)-(f).

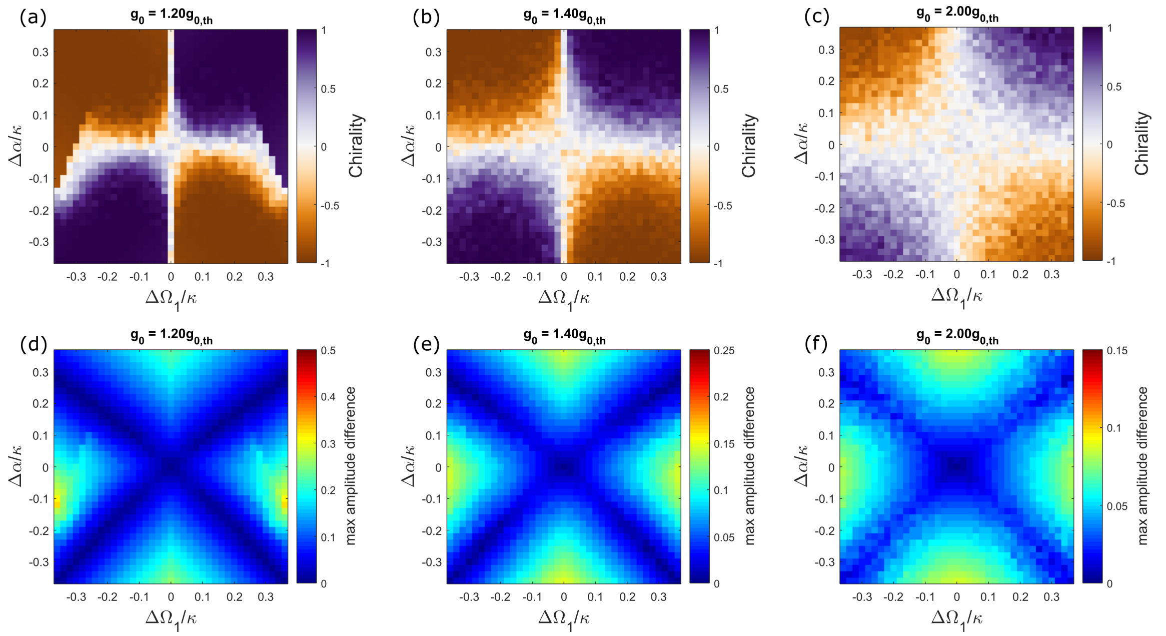


FIG. S10: (a) Chirality and (b) amplitude inhomogeneity of a system of coupled lasers as a function of $\Delta\Omega$ and $\Delta\alpha$, calculated by numerically solving the LRE for variuos values of $g_0$. Note the different colorbar range in panels (d)-(f).

## ASYMMETRIC ENERGY FLOW AND LASING THRESHOLD

The Hamiltonian (equation S5) is written in the basis of the individual lasers. To understand the effect of the complex potential on the dynamics of the vortex and antivortex modes, it is useful to transform the Hamiltonian to the basis of the vortex modes: uniform phase (U), vortex (V) and antivortex (AV). The transformation matrix is

$$T = \begin{pmatrix} 1 & 1 & 1 \\ 1 & e^{+\frac{2\pi}{3}i} & e^{-\frac{2\pi}{3}i} \\ 1 & e^{-\frac{2\pi}{3}i} & e^{+\frac{2\pi}{3}i} \end{pmatrix}$$

and the transformed Hamiltonian $\tilde{\mathcal{H}}$ is

$$\tilde{\mathcal{H}} = T^{-1}\mathcal{H}T = \begin{pmatrix} -2i & \kappa_1 \left(c\Delta\alpha - \Delta\Omega\right) & -\kappa_1^* \left(c\Delta\alpha + \Delta\Omega\right) \\ -\kappa_1^* \left(c\Delta\alpha + \Delta\Omega\right) & i & \kappa_1 \left(c\Delta\alpha - \Delta\Omega\right) \\ \kappa_1 \left(c\Delta\alpha - \Delta\Omega\right) & -\kappa_1^* \left(c\Delta\alpha + \Delta\Omega\right) & i \end{pmatrix} - \begin{pmatrix} \frac{1}{3}\Delta\alpha & 0 & 0 \\ 0 & \frac{1}{3}\Delta\alpha & 0 \\ 0 & 0 & \frac{1}{3}\Delta\alpha \end{pmatrix} \tag{S9}$$

where $c = 1.1547$ and $\kappa_1 = (0.25 + 0.144i)$.

The V and AV modes are coupled directly, and indirectly trough the extremely lossy U mode. The coupling between the V and AV modes is asymmetric and depends on the relation between $\Delta\alpha$ and $\Delta\Omega$. We also see the the round-trip loss of the V and AV mode is equal for every $\Delta\alpha$ and $\Delta\Omega$. In summary, we learn from this representation of $\mathcal{H}$ that the complex potential do not lift the loss degeneracy between the V an AV modes, but rather leads to an asymmetric energy flow between them.

The right term in $\tilde{\mathcal{H}}$ is just $-\frac{1}{3}\Delta\alpha$ multiplied by the identity matrix. This corresponds to a global shift in the loss of the three modes. In order to keep the ratio of the actual pumping rate and the threshold pumping rate constant during the measurement, a global linear gain correction of $\frac{1}{3}\Delta\alpha$ was added to all the lasers. The gain was applied in both the experiment and in the simulations.

## REFERENCES


[1] C. Tradonsky, I. Gershenzon, V. Pal, R. Chriki, A. A. Friesem, O. Raz, and N. Davidson, Science Advances **5** (2019), 10.1126/sciadv.aax4530, https://advances.sciencemag.org/content/5/10/eaax4530.full.pdf.
[2] S. Ngcobo, I. Litvin, L. Burger, and A. Forbes, Nature Communications **4**, 2289 (2013).
[3] V. Evtuhov and A. E. Siegman, Appl. Opt. **4**, 142 (1965).
[4] J. A. Arnaud, Appl. Opt. **8**, 189 (1969).
[5] I. Gershenzon, G. Arwas, S. Gadasi, C. Tradonsky, A. Friesem, O. Raz, and N. Davidson, Nanophotonics **9**, 4117 (2020).
[6] F. Rogister, K. S. Thornburg, L. Fabiny, M. Möller, and R. Roy, Phys. Rev. Lett. **92**, 093905 (2004).
[7] P. Peng, W. Cao, C. Shen, W. Qu, J. Wen, L. Jiang, and Y. Xiao, Nature Physics **12**, 1139 (2016).
